# Supplementary material for: On Robustness of Kernel Clustering
Source: arXiv:1606.01869 source file (2016-12-02)
Supplement: Supplementary file 1 [file supplementary.tex]

\documentclass{article}
\usepackage{xr}
\usepackage[final]{nips_2016}
\usepackage{xspace}

\usepackage[utf8]{inputenc} % allow utf-8 input
\usepackage[T1]{fontenc}    % use 8-bit T1 fonts
\usepackage{hyperref}       % hyperlinks
\usepackage{url}            % simple URL typesetting
\usepackage{booktabs}       % professional-quality tables
\usepackage{amsfonts}       % blackboard math symbols
\usepackage{nicefrac}       % compact symbols for 1/2, etc.
\usepackage{microtype}      % microtypography
\usepackage{graphicx}
\usepackage{subcaption}
\usepackage{color, comment}
\usepackage{bm, stmaryrd}

\usepackage{amsmath} % provides numberwithin (and lots more)
%\newtheorem{lemma}{Lemma}

% For algorithms
\usepackage{algorithm}
\usepackage{algorithmic}
\usepackage{footnote}
\usepackage{tablefootnote}
\usepackage{amsmath, amsthm, amssymb}

\numberwithin{lemma}{section}
\numberwithin{theorem}{section}

\numberwithin{equation}{section}
 %real numbers
 %natural numbers
 %complex numbers

\newcommand{\vertiii}[1]{{\left\vert\kern-0.25ex\left\vert\kern-0.25ex\left\vert #1 
    \right\vert\kern-0.25ex\right\vert\kern-0.25ex\right\vert}}

\title{Supplementary Material of\\
On Robustness of Kernel Clustering}

\author{
  Bowei Yan\\%\thanks{Use footnote for providing further
    %information about author (webpage, alternative
    %address)---\emph{not} for acknowledging funding agencies.} \\
  Department of Statistics and Data Sciences\\
  University of Texas at Austin
  %% examples of more authors
  \And
  Purnamrita Sarkar \\
    Department of Statistics and Data Sciences\\
  University of Texas at Austin
}

\externaldocument{nips16_kernel_clust}

\begin{document}
\maketitle
\appendix
\input{appendix}

\small{
\bibliographystyle{abbrv}
\bibliography{Bibliography}
}
\end{document}
